# Supplementary material for: Measurement-based quantum computation from Clifford quantum cellular automata
Source: arXiv:2312.13185 source file (2024-12-24)
Supplement: Supplementary file 1 [file appendix.tex]

\section{QCA-based quantum computation}

\subsection{Laurent formalism}

\subsection{Proving universality}

\section{MBQC as QCAQC}

\subsection{Mapping MBQC to QCAQC}

\subsection{Mapping QCAQC to MBQC}
